# Supplementary material for: Low-Latency Data Sharing in Erasure Multi-Way Relay Channels
Source: arXiv:1211.1044 source file (2013-07-30)
Supplement: Supplementary file 1 [file Appendix.tex]

Here, we calculate EEERs associated with MPW and OPPW. First, we find EEER for OPPW. The derivation of EEER for MPW has similar steps with some changes which are explained later.
